# Supplementary material for: Generating Counterfactual Explanations Under Temporal Constraints
Source: arXiv:2503.01792 source file (2025-03-03)
Supplement: Supplementary file 1 [file supplementary_material.tex]

\section{Supplementary material}

\subsection*{Proofs}
We prove the theorems witnessing correctness of our approach, i.e., that the crossover operator of Algorithm~\ref{alg:crossoveroperator}, as well as the mutation operators by the two strategies of Algorithm~\ref{alg:mutation_operator}, preserve the satisfaction of \LTLp formulae.

\thmalgoone*

\begin{proof}
Let $n = \length(\trace)$.
Upon inspection of Algorithm~\ref{alg:crossoveroperator}, one can see that every output $\trace_o$ produced by the algorithm  relates to the input trace $\trace$ as follows:
\begin{compactenum}
\item $\length(\trace_o) = \length(\trace) = n$;
\item for every $i \in \set{1,\ldots,n}$:
\begin{compactenum}
\item if $\trace(i) \in \activetasks{\varphi}$ then $\trace_o(i) = \trace(i)$;
\item if instead $\trace \not \in \activetasks{\varphi}$, that is, $\trace  \in \othertasks{\varphi}$, then $\trace_o(i) \in \othertasks{\varphi}$ as well -- equivalently, $\trace_o(i) \in \othertasks{\varphi}$ if and only if $\trace(i) \in \othertasks{\varphi}$.
\end{compactenum}
\end{compactenum}

By absurdum, imagine that $\trace_o \not \models \varphi$. Since, by property (1) above, $\length(\trace_o) = \length(\trace)$, this means that the violation must occur due to a mismatch in the evaluation of an atomic formula in some instant. Technically, there must exist $i \in \set{1,\ldots,n}$ and an atomic sub-formula $a \in \Sigma$ of $\varphi$ (which, by definition, requires $a \in \activetasks{\varphi}$) such that 
either:
\begin{compactenum}[(A)]
\item $\trace,i \models a$ and $\trace_o,i \not \models a$, or 
\item $\trace,i \not\models a$ and $\trace_o,i \models a$. 
\end{compactenum}

\noindent \emph{Case (A).} By the \LTLp semantics, we have $\trace(i) = a$ and $\trace_o(i) \neq a$. However, this is impossible: since $a$ belongs to $\activetasks{\varphi}$, then by property (2a) above, we have $\trace(i) = \trace_o(i)$.

\noindent \emph{Case (B).} By the \LTLp semantics, $\trace,i \not \models a$ if and only if $\trace(i) = b$ for some $b \in \Sigma \setminus \set{a}$. There are two sub-cases: either $b \in \activetasks{\varphi}\setminus \set{a}$, or $b \in \othertasks{\varphi}$. In the first sub-case, impossibility follows again from the fact that, by property (2a) above, since $b \in \activetasks{\varphi}$, then $\trace_o(i) = \trace(i) =b$, which implies $\trace_o,i \not\models a$. In the second sub-case, impossibility follows from the fact that $\trace_o(i)$ cannot be $a$, since by property (2b), the fact that $\trace(i) \in \othertasks{b}$ implies that also $\trace_o(i) \in \othertasks{b}$.
\end{proof}

\thmalgothree*

\begin{proof}
Correctness of \firstheur is proven analogously of Theorem~\ref{thm:crossover}. Correctness of \secondheur derives directly from the correspondence between the traces that satisfy $\varphi$, and the traces accepted by the \DFA of $\varphi$, $\aut_\varphi$. From the definition of \DFA acceptance, we have that since trace $\trace_o$ satisfies $\varphi$, there is a sequence $\istate, \ldots, \state_{n}$ of states of $\aut_\varphi$, such that:
\begin{inparaenum}[\itshape (i)]
\item the sequence starts from the initial state $\istate$ of $\aut$;
\item the sequence culminates in a last state, that is, $\state_{n} \in \fstates$;
\item for every $i \in \set{1,\ldots,n}$, we have $\trans(q_{i-1},\trace_o(i)) = q_{i}$. 
\end{inparaenum}

From Algorithm~\ref{alg:mutation_operator}, we have that trace $\trace_o$ is mutated through \secondheur by selecting an instant $i$, and allowing for replacing $\trace_o(i)$ with an activity $a$ returned from Algorithm~\ref{alg:safemoves}. From Algorithm~\ref{alg:safemoves}, we know that activity $a$ is returned if the following property holds: $\trans(\state_{i-1},a) = q_{i}$. This means that the mutated trace $\trace'_o$ that replaces $\trace_o(i)$ with $a$, and maintains the rest identical, is accepted by $\aut_\varphi$, with the same witnessing sequence of states $\istate, \ldots, \state_{n}$. From the correspondence between $\aut_\varphi$ and the \LTLp semantics of $\varphi$, we thus have $\trace'_o \models \varphi$.
\end{proof}

\subsection*{Technical material}
\subsubsection{Code for reproducing experiments}

The \emph{AAAI2025-temporal-constrained-counterfactuals} archive contains all the code used for re-running the experiments, including instructions on how to set up the environment and to install all the required dependencies. These instructions are provided in a Markdown file \emph{README.md}, detailing all the steps and commands for installation of all the packages detailed above.

\subsubsection{Code for results analysis}
The analysis of the results generated from the experiments is performed using a separate Jupyter notebook. This notebook includes code for loading and preprocessing the experimental results, performing statistical analysis such as calculating performance metrics, visualizing data, and comparing different methods. It also contains scripts for plotting results to visualize the performance and method comparisons.

This Jupyter notebook is included in the supplementary material and provides a comprehensive view of the analysis conducted, ensuring transparency and reproducibility of our results. For further details, the Jupyter notebook \emph{results\_analysis.ipynb} can be accessed as part of the supplementary material package.

\subsection*{Datasets}
Instructions to download the datasets used to run the experiments above are detailed in the README.MD file in the directory containing the code.

\subsection*{\LTLp formulas for each dataset}

For each dataset, we used different Linear Temporal Logic over Process Traces (\LTLp) formulas to check coverage at 10\%, 25\%, and 50\%. Below are the specific formulas used for each dataset:

\subsubsection*{BPIC2012 Dataset}

\begin{itemize}
    \item \textbf{10\%:}
    $
    \eventually(\text{osentcomplete}) \land \always(\text{osentcomplete} \rightarrow \neg(\text{aacceptedcomplete})\until(\text{wcompleterenaanvraagcomplete})) \land \eventually(\text{osentbackcomplete})
    $
    
    \item \textbf{25\%:}
    $
    \eventually(\text{osentcomplete}) \land \always(\text{osentcomplete} \rightarrow \neg(\text{aacceptedcomplete})\until(\text{wcompleterenaanvraagcomplete})) \land \eventually(\text{osentbackcomplete}) \land \always(\text{wcompleterenaanvraagstart} \rightarrow \eventually(\text{aacceptedcomplete})) \land (\eventually(\text{wnabellenoffertesstart}) \land \eventually(\text{wnabellenoffertescomplete})) \land (\eventually(\text{oselectedcomplete}) \lor \eventually(\text{wvaliderenaanvraagstart}))
    $
    
    \item \textbf{50\%:}
    $
    \eventually(\text{osentcomplete}) \land \always(\text{osentcomplete} \rightarrow \neg(\text{aacceptedcomplete})\until(\text{wcompleterenaanvraagcomplete})) \land \always(\text{wcompleterenaanvraagschedule} \rightarrow \eventually(\text{wcompleterenaanvraagstart})) \land (\eventually(\text{wnabellenoffertesstart}) \lor \eventually(\text{wnabellenoffertescomplete})) \land (\eventually(\text{oselectedcomplete}) \lor \eventually(\text{wvaliderenaanvraagstart})) \land \text{asubmittedcomplete} \land \eventually(\text{oselectedcomplete} \lor \text{apartlysubmittedcomplete}) \land \always(\text{ocreatedcomplete} \rightarrow \eventually(\text{osentbackcomplete})) \land \eventually(\text{afinalizedcomplete}) \lor \eventually(\text{apreacceptedcomplete}) \lor \eventually(\text{wafhandelenleadscomplete})
    $
\end{itemize}

\subsubsection*{BPIC17 Dataset}

\begin{itemize}
    \item \textbf{10\%:}
    $
    \text{acreateapplication} \land \neg(\text{aconcept})\until(\text{wcompleteapplication})
    $
    
    \item \textbf{25\%:}
    $
    \text{acreateapplication} \land \neg(\text{aconcept})\until(\text{wcompleteapplication}) \land (\eventually(\text{ocreateoffer}) \rightarrow \eventually(\text{wcallafteroffers})) \land \eventually(\text{wcompleteapplication})
    $
    
    \item \textbf{50\%:}
    $
    \text{acreateapplication} \land \neg(\text{aconcept})\until(\text{wcompleteapplication}) \land \always(\text{ocreateoffer} \rightarrow (\eventually(\text{wcallafteroffers}) \lor \eventually(\text{wvalidateapplication}))) \land (\eventually(\text{ocreated}) \rightarrow X(\text{osentmailandonline} \lor \text{osentonlineonly})) \land \always((\text{aincomplete} \lor \text{apending}) \rightarrow (X(\text{wcallincompletefiles}) \land \eventually(\text{wvalidateapplication})))
    $
\end{itemize}

\subsubsection*{Claim Management Dataset}

\begin{itemize}
    \item \textbf{10\%:}
    $
    \always(\text{contacthospital} \rightarrow X(\text{acceptclaim} \lor \text{rejectclaim}))
    $
    
    \item \textbf{25\%:}
    $
    \always(\text{contacthospital} \rightarrow X(\text{acceptclaim} \lor \text{rejectclaim})) \land \eventually(\text{createquestionnaire})
    $
    
    \item \textbf{50\%:}
    $
    (\eventually(\text{contacthospital}) \rightarrow \eventually(\text{highinsurancecheck})) \land \always(\text{preparenotificationcontent} \rightarrow X(\text{sendnotificationbyphone} \lor \text{sendnotificationbypost})) \land \always(\text{createquestionnaire} \rightarrow \eventually(\text{preparenotificationcontent})) \land \text{register}
    $
\end{itemize}

\subsection*{Predictive model Hyperparameter Configuration}

For the XGBoost predictive model, we defined the following hyperparameter search space:

\begin{itemize}

    \item The \emph{number of estimators} (\texttt{n\_estimators}) was selected from an integer range between 150 and 1000.

    \item The \emph{maximum} depth of each tree (\texttt{max\_depth}) was chosen as an integer value within the range of 3 to 30.
    
    \item The learning rate (\texttt{learning\_rate}) was selected from a continuous uniform distribution between 0.01 and 0.5.
    
    \item The \emph{subsample} ratio of the training instance (\texttt{subsample}) was chosen from a continuous uniform distribution between 0.5 and 1.    
\end{itemize}

The hyperparameter search was performed using the Hyperopt library, which allowed us to explore this search space efficiently to find the best configuration for our XGBoost model. We ran the hyperparameter search for 20 iterations for each dataset, prefix length and \LTLp combination.

\subsection*{Software and Tools Used for Compliance Checking with \LTLp Formula}

In our experiments, we utilized the \textbf{Declare4Py} Python package, which is available at \texttt{https://github.com/ \ ivanDonadello/Declare4Py}. This package was specifically employed to check compliance with Linear Temporal Logic over Finite Traces (\LTLf) formulas, readily applicable for \LTLp formulas.

The \textbf{Declare4Py} package relies on several external tools to perform its compliance checking:

\begin{enumerate}
    \item \textbf{LTLf2DFA}:
    \begin{itemize}
        \item The \textbf{LTLf2DFA} tool is necessary for converting \LTLp formulas into Deterministic Finite Automata (DFA), which is a crucial step in the compliance checking process.
        \item You can access \textbf{LTLf2DFA} at \texttt{https://github.com/ \ whitemech/LTLf2DFA/}
        \item \textbf{LTLf2DFA} itself has a dependency on the \textbf{MONA} tool.
    \end{itemize}
    
    \item \textbf{MONA}:
    \begin{itemize}
        \item \textbf{MONA} is a C++ package required by \textbf{LTLf2DFA} to handle the conversion process from \LTLp to DFA efficiently.
        \item \textbf{MONA} can be downloaded from \texttt{}{https://www.brics.dk/mona/download.html}.
    \end{itemize}
\end{enumerate}

These tools together enabled the effective compliance checking against the \LTLp formulas in our experimental setup.

\subsection*{Random Seed Settings}
For reproducibility of results in both hyperparameter optimization and counterfactual generation, random seed settings are crucial. In our experiments, we use the following random seed management approaches:

\begin{itemize}
    \item \textbf{Hyperparameter Optimization:} We use random seeds to ensure the reproducibility of the hyperparameter search process. This involves setting a fixed random seed when sampling hyperparameters, which is crucial for obtaining consistent and comparable results across different runs. For instance, we utilize the `np.random.seed(seed\_value)` function from NumPy to control randomness during hyperparameter tuning.
    \item \textbf{Counterfactual Generation:} Random seeds are also used to ensure reproducibility in the counterfactual generation process. This involves setting the random seed for various stochastic elements within the counterfactual generation algorithms. Again, we use `np.random.seed(seed\_value)` to achieve this.
\end{itemize}

The specific random seed values used in our experiments are detailed in the configuration settings of our code.
